# Supplementary material for: PlotQA: Reasoning over Scientific Plots
Source: arXiv:1909.00997 source file (2020-02-01)

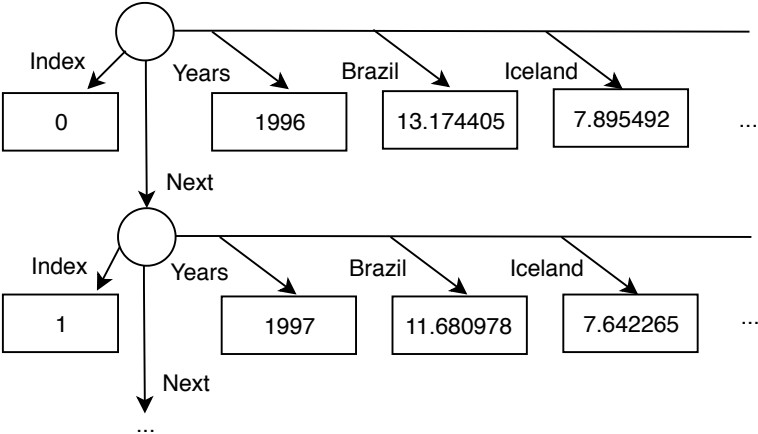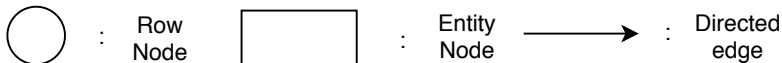

Supplement: Supplementary file 1 [file flow.pdf]
